# Supplementary material for: Local theory of the insulating state
Source: arXiv:1807.01063 ancillary file (2019-05-17)
Supplement: Supplementary file 1 [file supplementary.pdf]

# Local theory of the insulating state: Supplemental material

(Dated: 4-Apr-19)

## Tight-binding 1d Hamiltonians

Our 1d simulations adopt a nearest-neighbor 2-band tight-binding Hamiltonian with  $t = 1$ ; the site energies are  $\epsilon_j = (-1)^j \Delta$  (with  $\Delta = 0.25$ ) in the crystalline case, while in order to model a 1d Anderson insulator the string  $(-1)^j$  is replaced by a random string of  $\pm 1$ , chosen with equal (and uncorrelated) probability; in the latter case  $\tilde{\mathcal{L}}$ , as shown in the plots, is the average over 100 disorder realizations. Each of half-chains is up to 3,000 sites long; the LDOS and the “bulk” localization marker  $\tilde{\mathcal{L}}$  are evaluated over 60% of the sites, chosen in the central region of each half-chain.

## Tight-binding 2d Hamiltonians

Our 2d simulations adopt two similar Hamiltonians for the time-reversal-invariant cases (which are topologically trivial) and for the topological cases.

In order to address the topologically trivial cases we adopt a model tight-binding 2d Hamiltonian on a honeycomb lattice with two tight-binding sites per primitive cell with site energies  $\pm \Delta$  ( $\Delta = 2$ ), first-neighbor hoppings  $t_1 = 1$ , and second-neighbor hoppings  $t_2 = 1/3$ . The system is insulating at half filling ( $\mu = 0$ ) and metallic at any other filling. The localization marker for a homogeneous crystalline flake is displayed in the main text, Fig. 3, as a function of the flake size, for the insulating case only.

We have chosen the same Hamiltonian and  $\mu = -2.5$  in order to realize the metallic case. The resulting localization marker is shown here in Fig. 1; it clearly diverges linearly with the linear dimensions of the flake.

In order to model an heterojunction the bounded flake is cut through the center by a vertical interface: insulating to the left, metallic to the right, as in Fig. 2, top panel. We realize this by choosing  $\mu = 0$  and by adding a constant term equal to 2.5 to the onsite energies on the right half-flake. Fig. 2 (bottom) shows that the filling per cell is indeed 1/2 on the left half, and about 0.3 in the right half: the figure actually shows the site occupancy  $\langle \mathbf{r} | \mathcal{P} | \mathbf{r} \rangle$  along the horizontal line through the middle of the flake. Fig. 3 perspicuously shows that the trace of  $\tilde{\mathcal{L}}_{\alpha\beta}$  converges very fast to a constant value when the integration cell is chosen in the center of the insulating half-flake, and diverges linearly with size in the metallic case.

In order to address the topological cases we break time-reversal symmetry by switching from a real second-neighbor hopping  $t_2$  to a complex one  $t_2 = |t_2|e^{i\phi}$ . Our Hamiltonian thus becomes the (by now famous) Haldane

Hamiltonian [1], whose properties have been widely investigated. Notably, the half-filling ( $\mu = 0$ ) insulating state may be either trivial or topological, depending on the parameter values; for any other filling the system is metallic. The well known Haldane phase diagram at half filling is reproduced in Fig. 4. We focus here solely on the insulating topological case by choosing  $\phi = 0.25\pi$  and  $\Delta = 1/3$ , well into the topological region with Chern number  $C = -1$ .

We have also addressed a strongly disordered—and topologically nontrivial—flake by keeping  $\mu = 0$  and  $\phi = 0.25\pi$  as above, while the  $\Delta$  value at each site in the flake was chosen at random in the range  $[-1, 1]$  (again in the topological region), shown as a vertical segment in Fig. 4. With this choice anions and cations of various ionicity are randomly distributed.

We have validated the PBCs version of the localization marker, Eq. (7) in the main text, upon converting it into its tight-binding form. When we identify one of the two sites in the home cell with  $\mathbf{0}_\ell$ , the  $yy$  element becomes

$$\tilde{\mathcal{L}}_{yy} = \frac{1}{V_{\text{cell}}} \sum_{\mathbf{0}_\ell} \sum_{\mathbf{R}_m} (0_{\ell y} - R_{my})^2 |P(\mathbf{0}_\ell, \mathbf{R}_m)|^2, \quad (1)$$

where the PBCs ground-state projector  $P(\mathbf{0}_\ell, \mathbf{R}_m)$  is computed as a (discretized) reciprocal-space integral. Numerical summation of the series in Eq. (1) for the same Hamiltonian as used in the main text for the homogeneous insulating flake yields  $\tilde{\mathcal{L}}_{yy} = 0.0432$ , which is indeed one half of the converged value in Fig. 3 in the main text.

Next we switch to a superlattice made of slabs of A and B materials; the tight-binding local marker  $\tilde{\mathcal{L}}_{yy}$  is

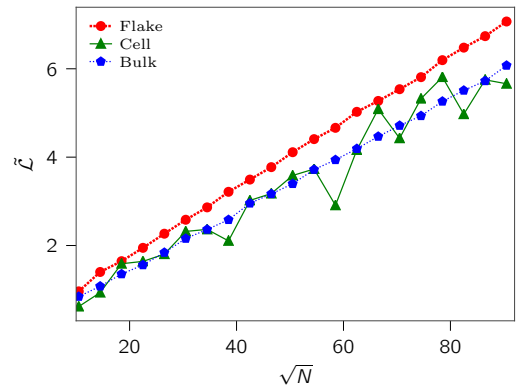

FIG. 1. (color online). Homogenous metallic flake. Cartesian trace of the localization tensor  $\mathcal{L}_{\alpha\beta}$  (labeled “Flake”), of our localization marker  $\tilde{\mathcal{L}}_{\alpha\beta}$  (labeled “Cell”), and an analogous formula evaluated over the “bulk region” (labeled “Bulk”), as a function of the flake size.

then defined as in Eq. (1), where the  $\mathbf{0}$  cell is chosen in the middle of either the A or the B regions. If the stacking axis is  $x$ , the insulating/metallic character of each region is detected via the convergence/divergence of  $\tilde{\mathcal{L}}_{yy}$  in the given  $x$ -region. Fig. 5 perspicuously shows that  $\tilde{\mathcal{L}}_{yy}$  converges very fast to a constant value when the integration cell is chosen in the center of the insulating slab, and diverges linearly with size in the metallic case, as in the OBCs case discussed earlier. The difference with respect to the OBCs case is that within PBCs the marker converges with respect to the number of  $\mathbf{R}_y$ -vectors and  $\mathbf{k}$ -points along the direction  $y$  that are used to compute Eq. (1). In the insulating region, the density matrix goes to zero exponentially for large  $\mathbf{R}_y$  and so the terms of Eq. (1). On the contrary, if we select a site in the metallic region then the corresponding terms in Eq. (1) do not go to zero for large values of  $\mathbf{R}_y$ , owing to the slow power-law decay of the ground-state projector in the  $y$  direction.

### First-principle implementation

We adopt the so-called Wannier-interpolation scheme [2] within density-functional theory (DFT): the Kohn-Sham Hamiltonian is projected onto a localized orthonor-

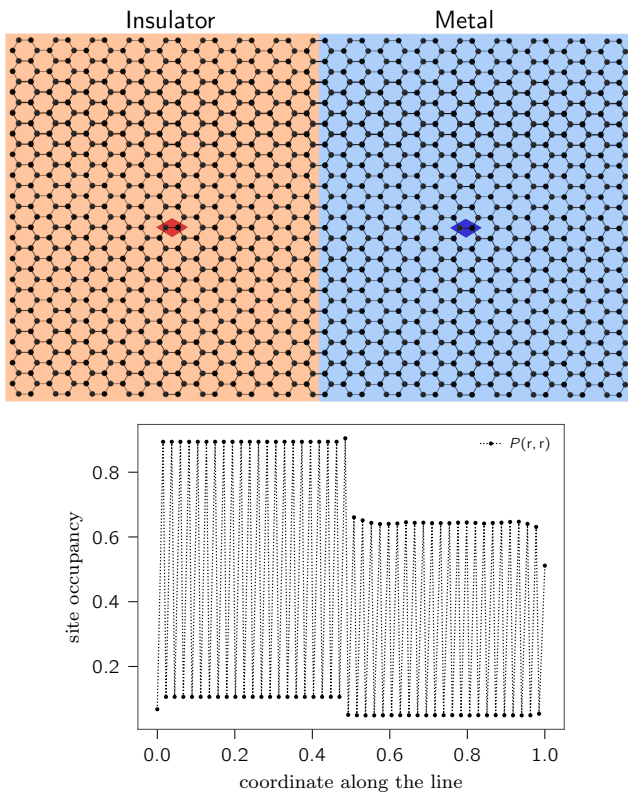

FIG. 2. Top panel: Heterojunction built of an insulating and a metallic half flake. Bottom panel: site occupancies for a 8190-site flake.

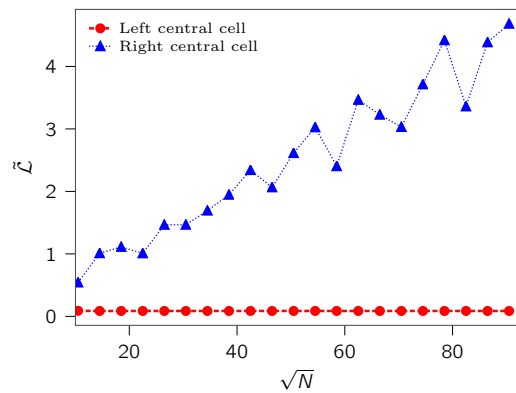

FIG. 3. (color online). Results for an heterojunction built of an insulating and a metallic half flake. Cartesian trace of  $\tilde{\mathcal{L}}_{\alpha\beta}$  evaluated at the center of the left (insulating) and right (metallic) half flakes as a function of size.

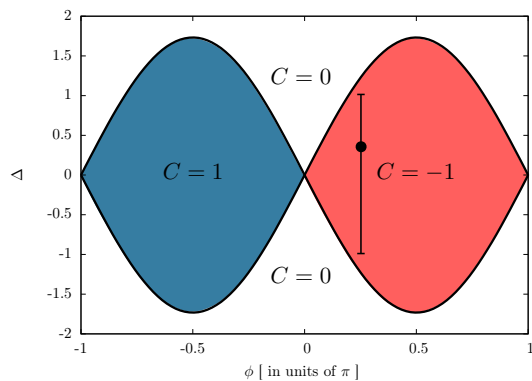

FIG. 4. Phase diagram of the Haldane model Hamiltonian at half filling ( $\mu = 0$ ), for  $t_1 = 1$  and  $|t_2| = 1/3$ , in the  $\phi$ ,  $\Delta$  variables. The coloured regions are the topological ones, with Chern number  $C = \pm 1$ . The dot indicates the choice performed for addressing the crystalline case, while for the disordered case the parameters are randomly chosen in the vertical segment.

mal basis set; the number of basis functions in each crystal cell (in either the A or B regions) is finite. The basis functions are obtained as supercell MLWFs (maximally localized Wannier functions) for a redundant set of bands, up to energies higher than the actual Fermi energy. The projection has been proved to be very successful in several circumstances [2]: in particular it accurately maps the Kohn-Sham Hamiltonian on a tight-binding-like one, capable of describing both insulating and metallic systems.

In the main text we have labelled the basis set as  $|\chi_{\mathbf{R}_\ell}\rangle$ , where  $\mathbf{R}_\ell$  is the orbital center. We have therefore a lattice of centers, *not* a lattice of nuclei; in particular, different  $\mathbf{R}_\ell$  may occupy the same position in space.

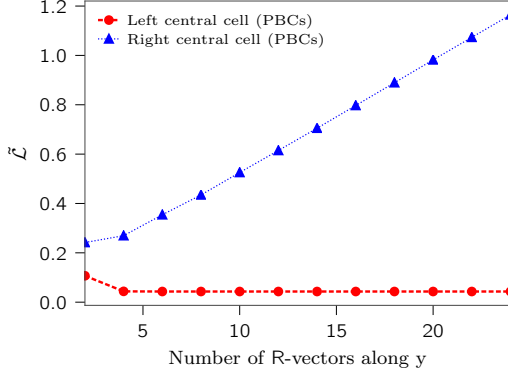

FIG. 5. (color online). Results for a periodic heterostructure built of alternating insulating and metallic slabs, but with a superlattice unit cell made of 160 sites along the horizontal axis. Cartesian trace of  $\tilde{\mathcal{L}}_{yy}$  evaluated at the center of the insulating and metallic slabs as a function of the  $\mathbf{R}$ -vectors and  $\mathbf{k}$ -points, along the direction  $y$ , used to compute the density matrix and Eq. (1).

The matrix elements of the ground-state projector over the basis are obtained as

$$P(\mathbf{0}_\ell, \mathbf{R}'_m) = \frac{V}{(2\pi)^3} \sum_n \int d\mathbf{k} C_{nl}^{\mathbf{k}} C_{nm}^{\mathbf{k}*} e^{i\mathbf{k} \cdot (\mathbf{R}'_m - \mathbf{0}_\ell)}, \quad (2)$$

the index  $n$  runs over the occupied bands, and  $C_{nl}^{\mathbf{k}}$  are the coefficients of the Bloch eigenstates over the basis, for a given  $\mathbf{k}$ -point.

The integral is performed over the Brillouin zone of the supercell on a discrete  $\mathbf{k}$ -point set. The convergence is checked with respect to the number of points along  $k_y$ , while the number of points along  $k_x$  and  $k_z$  is kept fixed.

DFT calculations are performed using plane waves and pseudopotentials as implemented in the PWscf code of the Quantum ESPRESSO distribution [3, 4]. We use the Perdew-Burke-Ernzerhof (PBE) [5] functional with the Standard Solid State Pseudopotentials (SSSP) Efficiency (version 1.0) library and cutoffs [6–8]. We build a tight-binding model in a basis of MLWFs that reproduces the band structure of the occupied states and some of the lowest lying empty states [2]. MLWFs are obtained using WANNIER90 [9].

### Towards many-body wavefunctions and Mott insulators

In the main text we discuss the case of independent electrons in crystalline and disordered potentials, while here we outline the fundamental steps to generalize the localization marker to many-body wavefunctions, as in the case of Mott insulators.

We consider an  $N$ -electron system, where  $N$  is even, and a singlet ground state  $\Psi$ . We introduce the one-body

and two-body densities

$$n(\mathbf{r}_1) = N \sum_{\sigma_1} \int d\mathbf{x}_2 d\mathbf{x}_3 \dots d\mathbf{x}_N |\Psi(\mathbf{x}_1, \dots, \mathbf{x}_N)|^2, \quad (3)$$

$$n^{(2)}(\mathbf{r}_1, \mathbf{r}_2) = N(N-1) \sum_{\sigma_1, \sigma_2} \int d\mathbf{x}_3 \dots d\mathbf{x}_N |\Psi(\mathbf{x}_1, \dots, \mathbf{x}_N)|^2, \quad (4)$$

where  $\mathbf{x}_i = (\mathbf{r}_i, \sigma_i)$  represents the space and spin coordinates of the  $i$ -th electron. Following Ref. [10], we write the localization tensor in OBCs as

$$\mathcal{L}_{\alpha\beta} = \frac{1}{2V} \int d\mathbf{r} d\mathbf{r}' (\mathbf{r} - \mathbf{r}')_\alpha (\mathbf{r} - \mathbf{r}')_\beta \cdot \quad (5)$$

$$\cdot (n(\mathbf{r})n(\mathbf{r}') - n^{(2)}(\mathbf{r}_1, \mathbf{r}_2)). \quad (6)$$

The last equation can be understood as a prescription for measuring the second cumulant moment of the exchange-correlation hole [10], defined as

$$n_{xc}(\mathbf{r}_1, \mathbf{r}_2) = n^{(2)}(\mathbf{r}_1, \mathbf{r}_2) - n(\mathbf{r}_1)n(\mathbf{r}_2). \quad (7)$$

Following the same strategy that led to Eq. (6) of the main text, we can now define the localization marker as the real symmetric part of

$$\tilde{\mathcal{L}}_{\alpha\beta} = \frac{1}{2V_{cell}} \int_{V_{cell}} d\mathbf{r} \int d\mathbf{r}' (\mathbf{r} - \mathbf{r}')_\alpha (\mathbf{r} - \mathbf{r}')_\beta \cdot \quad (8)$$

$$\cdot (n(\mathbf{r})n(\mathbf{r}') - n^{(2)}(\mathbf{r}_1, \mathbf{r}_2)) \quad (9)$$

where the integration cell of the outer integral can lie in a metallic or insulating region as discussed in the main text. Although the calculation of  $n^{(2)}(\mathbf{r}_1, \mathbf{r}_2)$  is indeed a formidable task, some of the computational shortcuts introduced in this work for independent electrons can also be generalised to the many-body framework. In particular, we can use many-body Wannier functions as an optimal basis for interpolation and study the asymptotic behaviour of the kernel of the exchange-correlation hole, similarly to the procedure that has been developed for the one-body density matrix in the first-principle implementation. In addition, one could benefit from a recent alternative approach to compute the macroscopic polarization of correlated systems developed in Ref. [11]. There, Requist and Gross introduce an approximate formula for the many-body polarization by summing the geometric phases of natural orbitals with fractional occupations. Their formula maintains the simplicity of the independent-electron formulation and, at the same time, potentially capture the dominant correlation effects. This is carried out by adopting the expression for polarization by King-Smith and Vanderbilt [12] while replacing the periodic part of the Bloch orbital  $u_{n\mathbf{k}}(\mathbf{r})$  with

$$u_{n\mathbf{k}}(\mathbf{r}) \longrightarrow \sqrt{f_{n\mathbf{k}}} e^{i\zeta_{n\mathbf{k}}} u_{n\mathbf{k}}(\mathbf{r}), \quad (10)$$

where  $f_{n\mathbf{k}}$  is the occupation number and  $\zeta_{n\mathbf{k}}$  is a fundamental phase factor chosen from the stationary conditions on the total energy [11]. A similar procedure can be employed for the localization marker that we introduced in the present work, leading to a formula that would locally assess the metallic/insulating state of inhomogeneous correlated materials.

- 
- [1] F. D. M. Haldane, Phys. Rev. Lett. **61**, 2015 (1988).
  - [2] N. Marzari, A. A. Mostofi, J. R. Yates, I. Souza, and D. Vanderbilt, Rev. Mod. Phys. **84**, 1419 (2012).
  - [3] P. Giannozzi, S. Baroni, N. Bonini, M. Calandra, R. Car, C. Cavazzoni, D. Ceresoli, G. L. Chiarotti, M. Cococcioni, I. Dabo, A. Dal Corso, S. de Gironcoli, S. Fabris, G. Fratesi, R. Gebauer, U. Gerstmann, C. Gougousis, A. Kokalj, M. Lazzeri, L. Martin-Samos, N. Marzari, F. Mauri, R. Mazzarello, S. Paolini, A. Pasquarello, L. Paulatto, C. Sbraccia, S. Scandolo, G. Sclauzero, A. P. Seitsonen, A. Smogunov, P. Umari and R. M. Wentzcovitch, J. Phys.: Condens. Matter **21**, 395502 (2009)
  - [4] P. Giannozzi, O. Andreussi, T. Brumme, O. Bunau, M. Buongiorno Nardelli, M. Calandra, R. Car, C. Cavazzoni, D. Ceresoli, M. Cococcioni, N. Colonna, I. Carnimeo, A. Dal Corso, S. de Gironcoli, P. Delugas, R. A. DiStasio Jr., A. Ferretti, A. Floris, G. Fratesi, G. Fugallo, R. Gebauer, U. Gerstmann, F. Giustino, T. Gorni, J. Jia, M. Kawamura, H-Y. Ko, A Kokalj, E. Kkbenli, M. Lazzeri, M. Marsili, N. Marzari, F. Mauri, N. L. Nguyen, H-V. Nguyen, A. Otero-de-la-Roza, L. Paulatto, S. Ponc , D. Rocca, R. Sabatini, B. Santra, M. Schlipf, A. P. Seitsonen, A. Smogunov, I. Timrov, T. Thonhauser, P. Umari, N. Vast, X. Wu and S. Baroni, J. Phys.: Condens. Matter **29** 46590 (2017)
  - [5] J. P. Perdew, K. Burke, and M Ernzerhof, Phys. Rev. Lett. **77**, 3865 (1996)
  - [6] G. Prandini, A. Marrazzo, I. E. Castelli, N. Mounet and N. Marzari, npj Computational Materials **4**, 72 (2018)
  - [7] A. Dal Corso, Comput. Mater. Sci. **95**, 337 (2014)
  - [8] E. Kucukbenli, M. Monni, B. I. Adetunji, X. Ge, G. A. Adebayo, N. Marzari, S. de Gironcoli, A. Dal Corso, arXiv:1404.3015 [cond-mat.mtrl-sci] (2014)
  - [9] A. A. Mostofi, J. R. Yates, G. Pizzi, Y.-S. Lee, I. Souza, D. Vanderbilt and N. Marzari, Comput. Phys. Commun. **185**, 2309 (2014)
  - [10] R. Resta, J. Chem. Phys. **124**, 104104 (2006)
  - [11] R. Requist and E. K. U. Gross, J. Phys. Chem. Lett., **9** (24) (2018)
  - [12] D. Vanderbilt, *Berry Phases in Electronic Structure Theory* (Cambridge University Press, Cambridge, 2018).
